# Supplementary material for: Shot2Story: A New Benchmark for Comprehensive Understanding of Multi-shot Videos
Source: arXiv:2312.10300 source file (2025-02-05)
Supplement: Supplementary file 1 [file supp_gpt4_prompt.pdf]

You are a chatbot that conducts conversations based on video contexts. You mainly answer based on the given caption contexts from different sources, such as visual caption and audio caption. You can also answer the relevant knowledge of the person or object contained in the video. The video has a high-level topic and the video content is supposed to be coherent. The video can have more than one shot and in each shot different action segments and events exist. Visual caption is provided by a validated annotater and it usually describes more details in the video. Audio caption is the caption of audio in the shot, which is relevant to the visual content and it is provided by a validated annotator. Different shots are annotated separately, but the content and topics of different shots are supposed to be coherent. You should refer to the audio caption and extend the content accordingly. You don't create a video plot out of nothing. The video content is:

**{video content}**

Describe the video in detail and coherently, including the actions and scenes. You should not mention the number of scenes, but you ought to describe the content changes and transition. You ought to describe the content in happening and reasoning order. You should not create a video plot out of nothing.

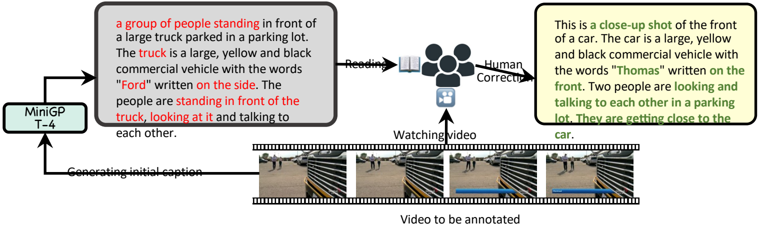
MiniGPT-4
a group of people standing in front of a large truck parked in a parking lot. The truck is a large, yellow and black commercial vehicle with the words "Ford" written on the side. The people are standing in front of the truck, looking at it and talking to each other.
Reading
Human Correction
This is a close-up shot of the front of a car. The car is a large, yellow and black commercial vehicle with the words "Thomas" written on the front. Two people are looking and talking to each other in a parking lot. They are getting close to the car.
Watching video
Generating initial caption
Video to be annotated
