# Supplementary material for: Shot2Story: A New Benchmark for Comprehensive Understanding of Multi-shot Videos
Source: arXiv:2312.10300 source file (2025-02-05)
Supplement: Supplementary file 2 [file supp_gpt4_video_prompt.pdf]

The video has **4** shots. It has **15.8 seconds** in total.
The first action segment starts from **0.0** seconds to **6.5** seconds.
Visual caption of this clip is: **It's a man in a kitchen chopping something with a knife. The man is wearing a tee shirt with the number 19 on it. He seems to hurt himself and appears in pain. The video is in black and white. The yellow words "DON'T RISK IT" appear on the screen. Then the scene changes to a bowl of guacamole with chips on the side. The video also shows the package.**
The audio caption of this clip is: **In the audio, the background voice says don't risk getting injured from cutting up avocados.**

The second action segment starts from **6.5** seconds to **10.5** seconds.
Visual caption of this clip is: **It's a close-up of a person scooping avocado out with a spoon on a wooden cutting board. There is also a white bowl next to it.**
The audio caption of this clip is: **In the audio, the background voice says the product is refrigerated and pre-scooped for the customers.**

The third action segment starts from **10.5** seconds to **13.5** seconds.
Visual caption of this clip is: **It's a woman in a pink shirt with a cast on her arm. She holds her thumb up with the injured arm. The word "SWEET" in purple is typed on the screen.**
The audio caption of this clip is:

The forth action segment starts from **13.5** seconds to **15.8** seconds.
Visual caption of this clip is: **It's a bowl of guacamole with chips on the side. There is a plastic container of guacamole with a purple package next to it.**
The audio caption of this clip is:

The ASR of the video is: **ASR content**

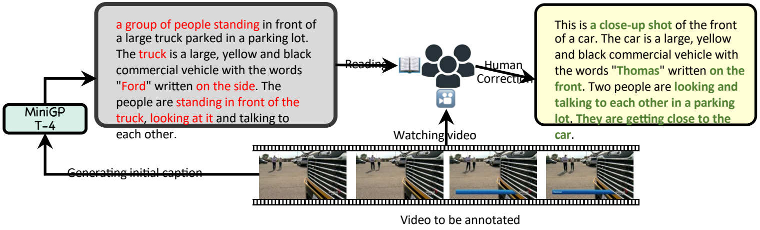

a group of people standing in front of a large truck parked in a parking lot. The truck is a large, yellow and black commercial vehicle with the words "Ford" written on the side. The people are standing in front of the truck, looking at it and talking to each other.
MiniGPT-4
Reading
Human Correction
This is a close-up shot of the front of a car. The car is a large, yellow and black commercial vehicle with the words "Thomas" written on the front. Two people are looking and talking to each other in a parking lot. They are getting close to the car.
Watching video
Generating initial caption
Video to be annotated
