# Supplementary material for: Shot2Story: A New Benchmark for Comprehensive Understanding of Multi-shot Videos
Source: arXiv:2312.10300 source file (2025-02-05)

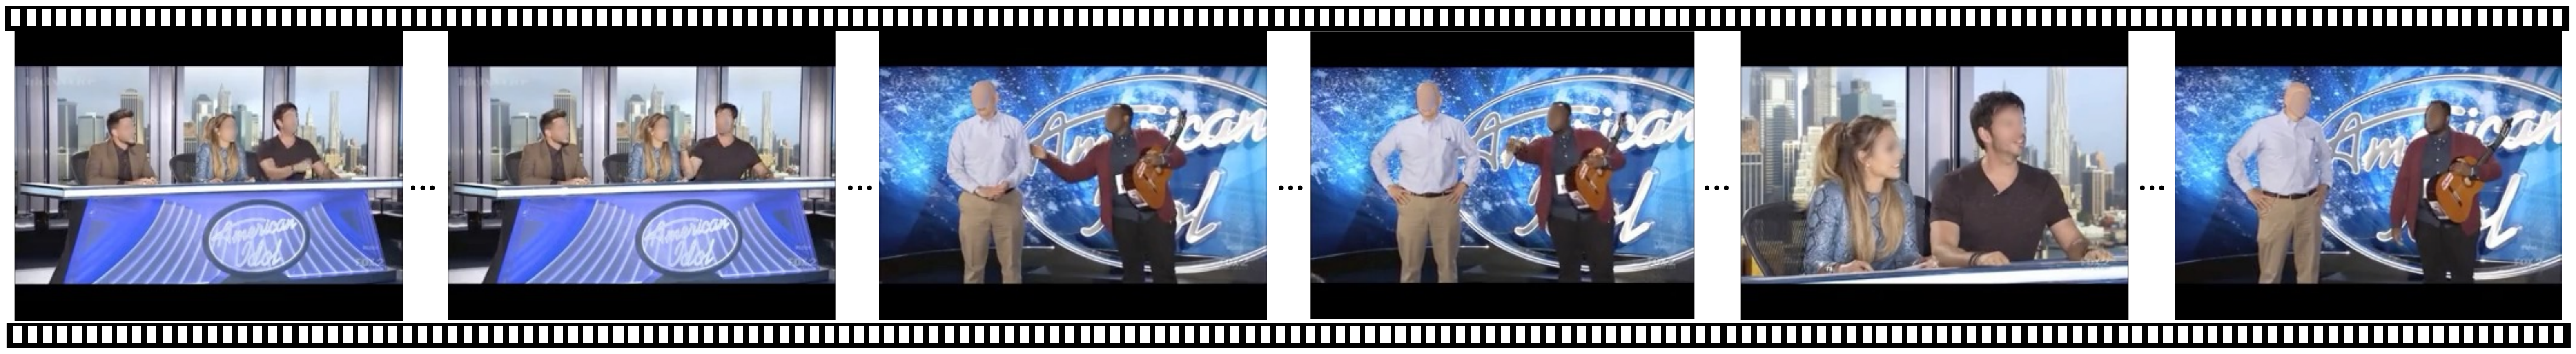

video7089.mp4

***SUM-shot*** video summarization:

the video begins with a man in a black shirt and a woman in a blue shirt sitting behind a blue and silver-colored table with a city skyline in the background. they are engaged in a conversation, with the man occasionally clapping his hands. the scene then transitions to two men standing next to a large screen with american idol written on it. one man, dressed in a white shirt and black pants, picks up a guitar and starts playing. the other man, wearing a black shirt and khaki pants, claps his hands and smiles. in the final scene, the man in the white shirt and black pants continues to play the guitar, while the woman in the blue and silver-colored shirt looks at the camera. the man in the black shirt and khaki pants claps his hands and smiles. the video captures the interactions and performances of these individuals in front of the american idol backdrop.

**Questions**:

Q1: who speaks to tv show judges?
Q2: who do three judges talk to?
Q3: what is a black male laughing on?
Q4: what talks to a performer?
Q5: what did the man audition for?
Q6: who does a panel talk to?
Q7: what do judges talk on?
Q8: what shows judges of a singing competition?
Q9: how many contestants are standing before the judges at american idol?
Q10: what is going on?

**Answers**:

GT1: person
GT2: contestant
GT3: idol
GT4: panel
GT5: idol
GT6: performer
GT7: idol
GT8: video
GT9: two
GT10: reality

**Vicuna answers using summaries & GPT evaluation**:

A1: Based on the video description, it is not clear who is speaking to TV show judges. ❌

A2: The three judges in the video are the man in the black shirt and khaki pants, who claps his hands and smiles, and the woman in the blue and silver-colored shirt, who looks at the camera. ✅

A3: I'm sorry, but I cannot identify a specific person laughing in the video, as there is no mention of a person laughing in the description. The video appears to be focused on the interactions and performances of the individuals in front of the American Idol backdrop. ❌

A4: The man in the white shirt and black pants is a performer. ❌

A5: The man in the white shirt and black pants auditioned for American Idol. ✅

A6: Based on the video, it appears that a panel talk is happening between the man in the black shirt and the woman in the blue shirt, who are sitting behind a table with a city skyline in the background. The man occasionally claps his hands, and the scene transitions to two men standing next to a large screen with \"American Idol\" written on it. One man, dressed in a white shirt and black pants, picks up a guitar and starts playing, while the other man, wearing a black shirt and khaki pants, claps his hands and smiles. In the final scene, the man in the white shirt and black pants continues to play the guitar, while the woman in the blue and silver-colored shirt looks at the camera. The man in the black shirt and khaki pants claps his hands and smiles. ❌

A7: Judges talk about performances in front of the American Idol backdrop. ✅

A8: The video shows judges of a singing competition. ✅

A9: Two contestants are standing before the judges at American Idol. ✅

A10: It appears that the video is a behind-the-scenes look at a recording session for a musical performance, possibly for a talent competition such as American Idol. The individuals shown in the video are a group of musicians who are preparing for a performance in front of a panel of judges. The man in the black shirt and khaki pants is likely a music producer or judge, while the man in the white shirt and black pants is likely a contestant on the show. The woman in the blue and silver-colored shirt is likely another member of the group or a crew member. ❌

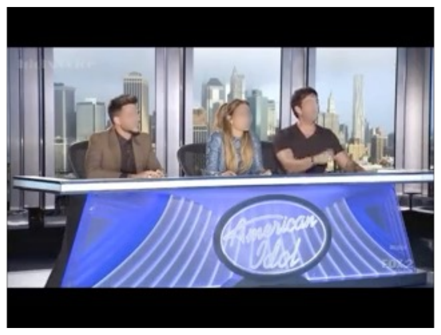
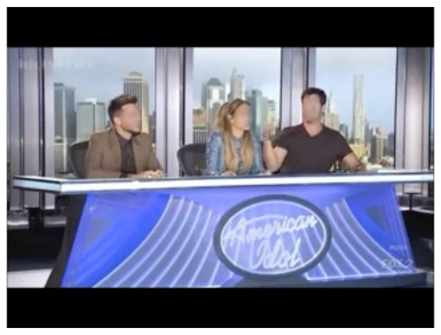
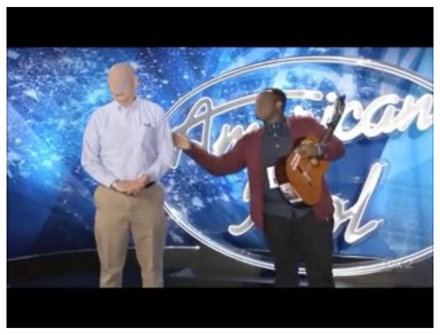
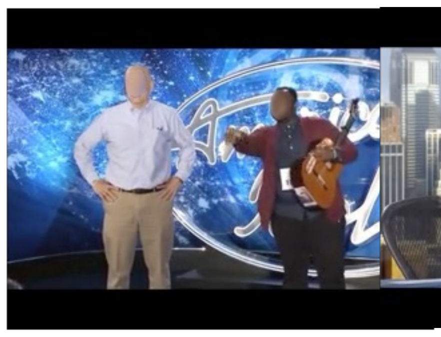
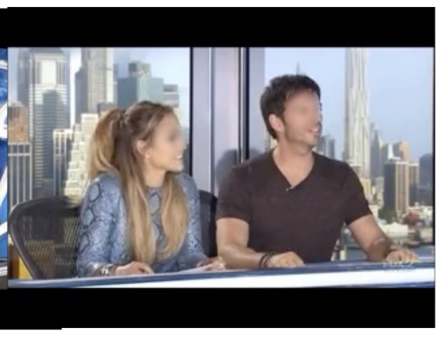
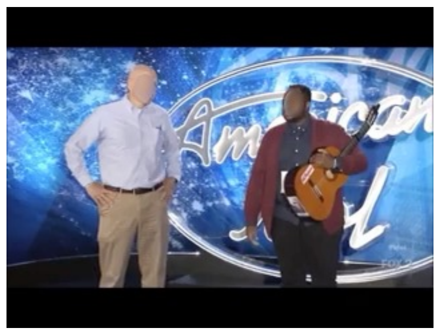

Supplement: Supplementary file 3 [file supp_qa_summary_msrvtt.pdf]
