# Supplementary material for: Shot2Story: A New Benchmark for Comprehensive Understanding of Multi-shot Videos
Source: arXiv:2312.10300 source file (2025-02-05)
Supplement: Supplementary file 4 [file supp_anno_process.pdf]

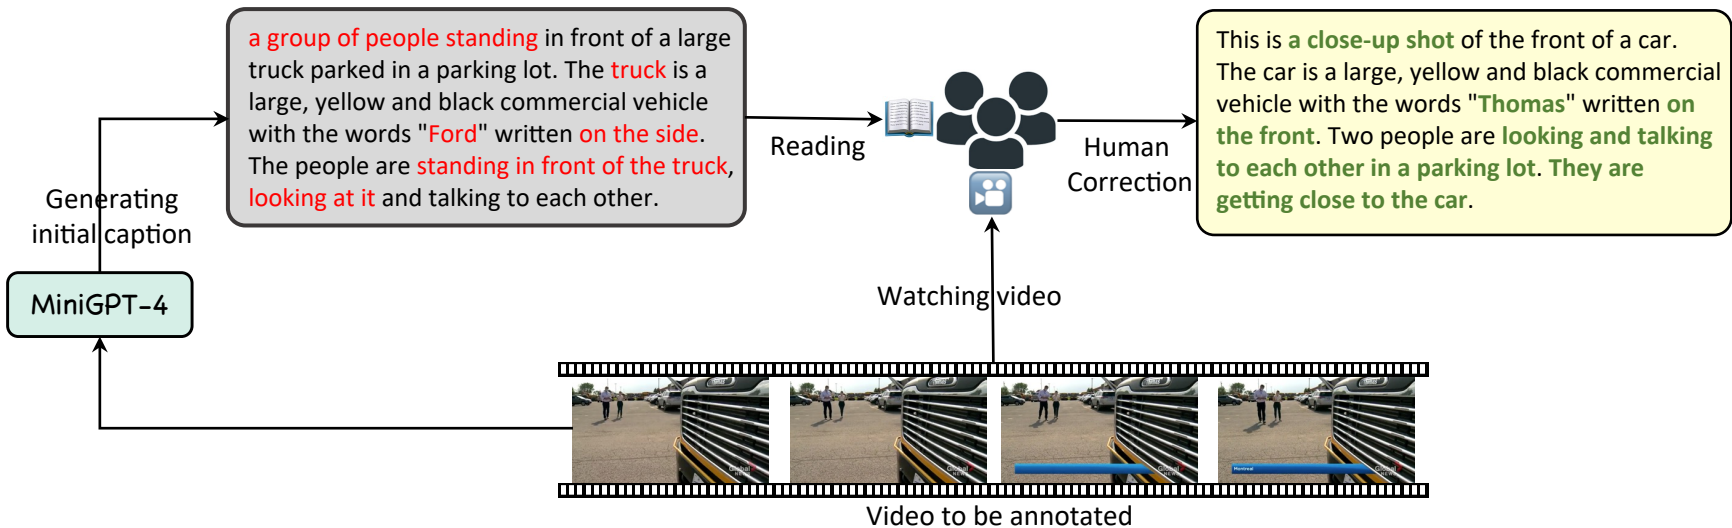

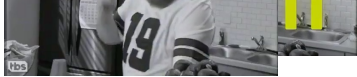

shot 1

⋮

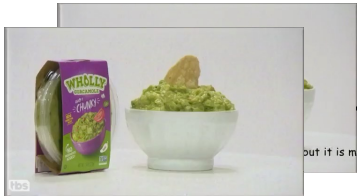

shot 4

Input to LLM

CLIP  
encoder

Q-Former

CLIP  
encoder

Q-Former

The second shot is ... The third shot is ... The fourth shot is

$\mathbf{v}_1^4$  ...  $\mathbf{v}_{N_s}^4$

In the audio, I hear that:

"Have you suffered an avocado related injury, dont risk it holy guacamole is refrigerated and pre scooped for your protection."

Large Language Model

Multi-shot Video summary

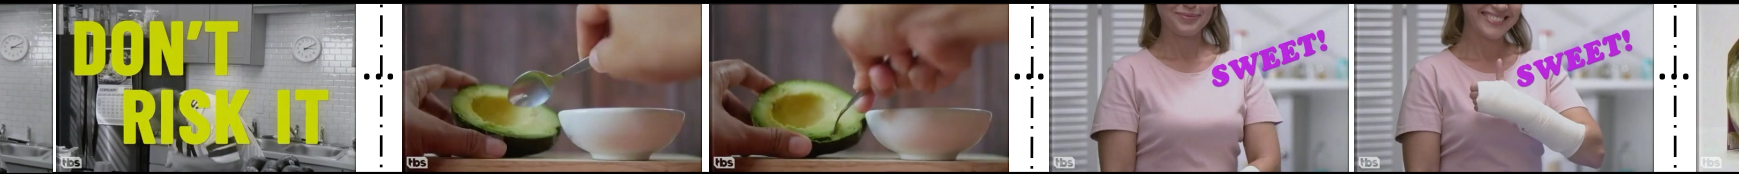

a kitchen, wearing a T-shirt with the number 19 on it. He is chopping something with a knife, but he seems to h  
and white for dramatic effect. As a cautionary message, the yellow words "DON'T RISK IT" appear on the scre  
on the side, and the package of the product is also shown. The audio during this segment warns viewers not to r
