# Supplementary material for: Shot2Story: A New Benchmark for Comprehensive Understanding of Multi-shot Videos
Source: arXiv:2312.10300 source file (2025-02-05)

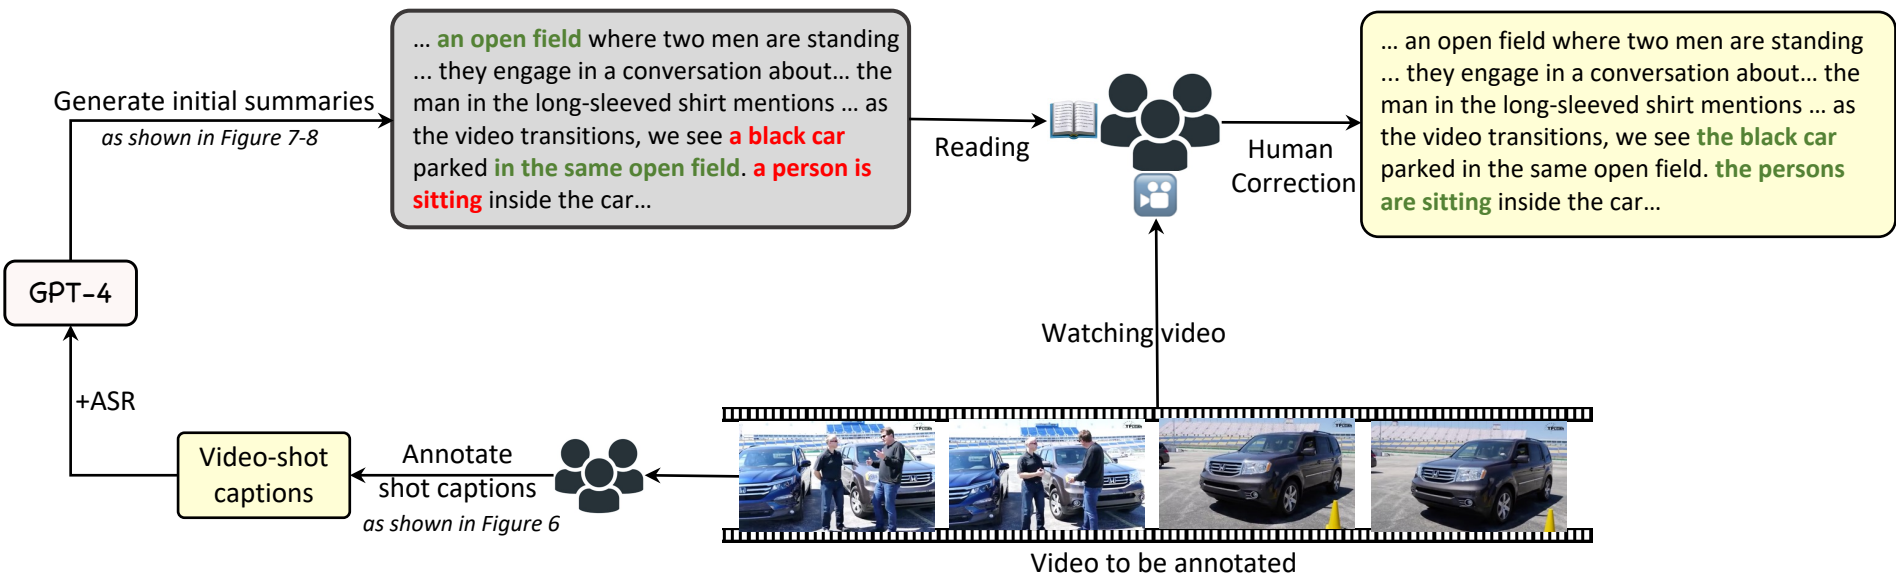

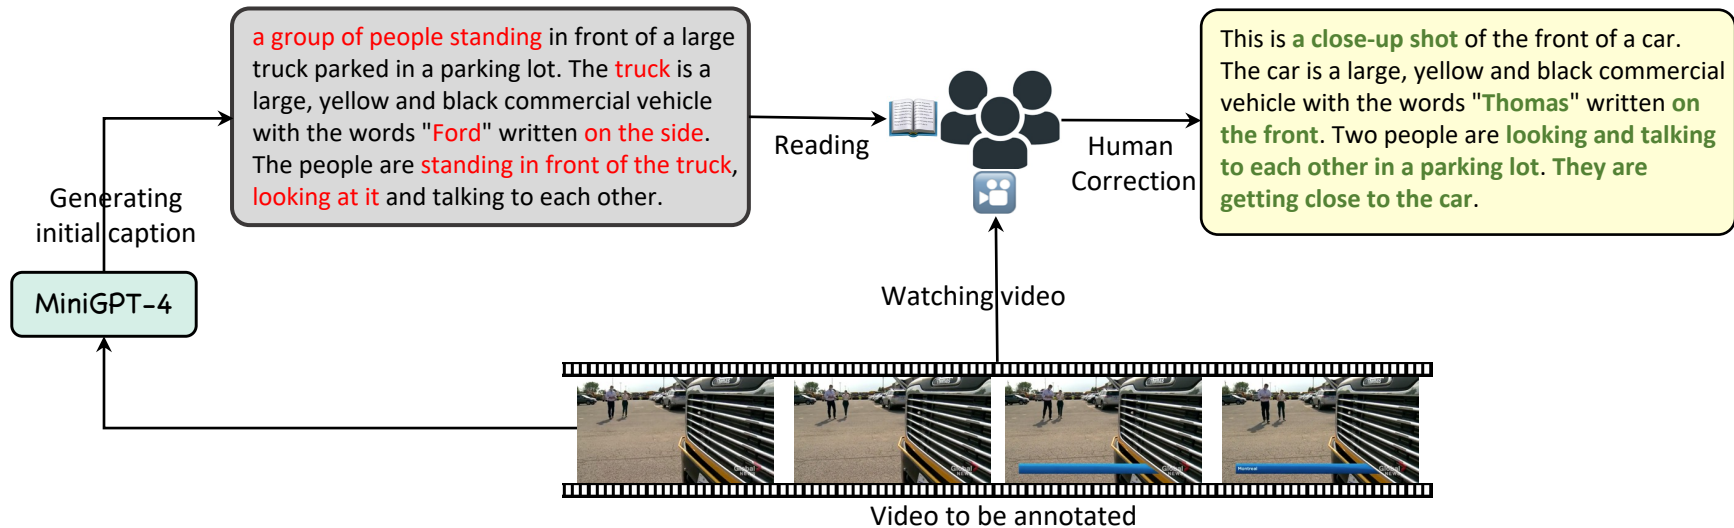

Supplement: Supplementary file 5 [file supp_referring_correction.pdf]
