# Supplementary material for: Shot2Story: A New Benchmark for Comprehensive Understanding of Multi-shot Videos
Source: arXiv:2312.10300 source file (2025-02-05)

Random one during training:

1. The audio transcripts are: **{asr}**. Describe the audio content of this video in detail.
2. In the audio, I hear that: **{asr}**. Take a look at this video clip and describe what you notice in the audio.
3. Based on the audio, the speech contents are: **{asr}**. Please provide a detailed description of the audio in the video.
4. From the audio, I gather the content that: **{asr}**. Could you describe the contents of the audio in this video for me?

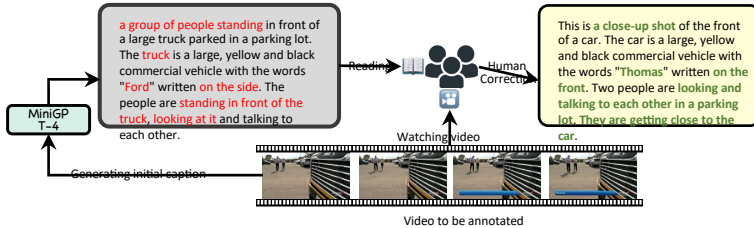

Supplement: Supplementary file 6 [file supp_shot_audio_cap.pdf]
