# Supplementary material for: Shot2Story: A New Benchmark for Comprehensive Understanding of Multi-shot Videos
Source: arXiv:2312.10300 source file (2025-02-05)

I need your help to identify a specific object, place, person and way in the video based on its description. You must answer my question concisely. The answer is definitely contained in the provided video description. Video content is:

**{video summary}**

You should answer the question concisely. Based on the video, please answer **{video question}**

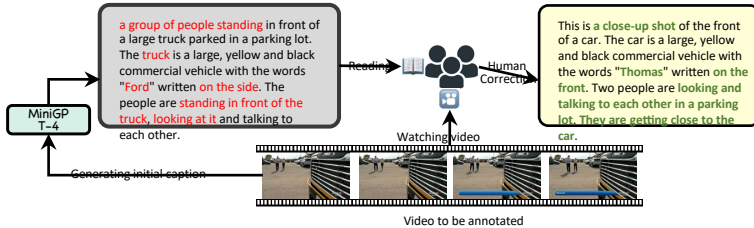

Supplement: Supplementary file 7 [file supp_vicuna_qa.pdf]
