# Supplementary material for: Shot2Story: A New Benchmark for Comprehensive Understanding of Multi-shot Videos
Source: arXiv:2312.10300 source file (2025-02-05)

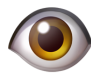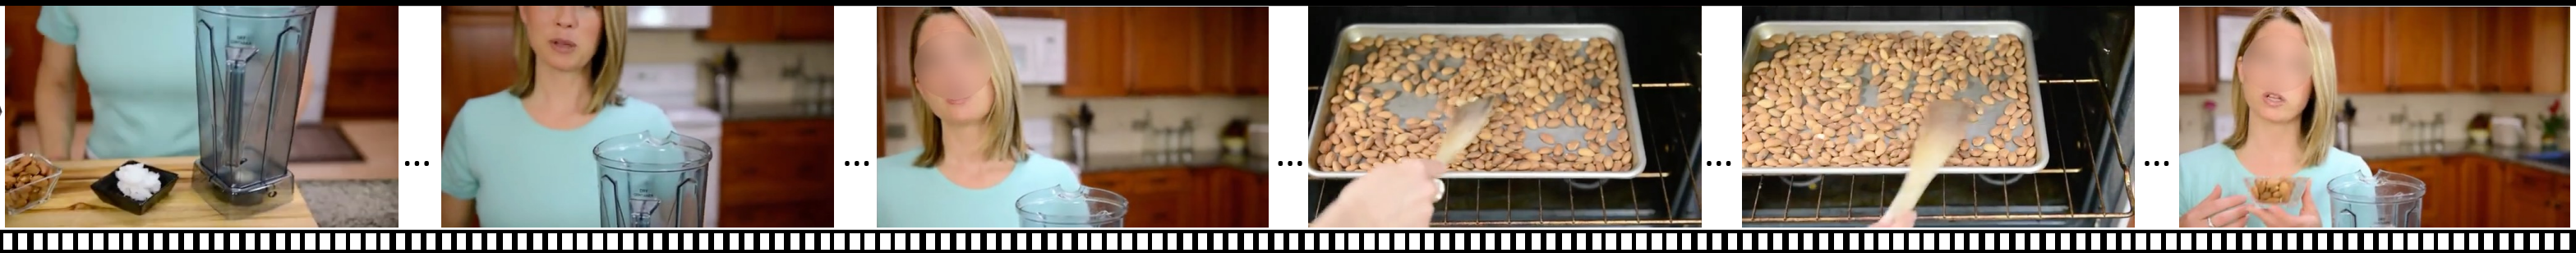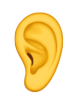

**Human speech:** However, there are a couple of tricks that you need to know in order to be successful. The first is that you must roast your almonds that helps to bring out not only the flavors but the oil as well.

**SUM-text** video summarization:

the video begins with a woman in a green t-shirt standing in a kitchen, holding a blender and engaging in a conversation with the camera. a bowl of almonds is situated on the counter in front of her, indicating that she is likely discussing a recipe that involves almonds. as the video progresses, the scene transitions to a person using a spatula to mix the almonds in a baking tray that is placed in an oven. this suggests that the woman is demonstrating a cooking process, possibly preparing a dish that involves roasted almonds. In the final part of the video, the woman, now wearing a blue top, is seen holding a bowl of almonds and continuing her conversation with the camera. a blender is visible in front of her, suggesting that she is discussing a recipe that involves blending the almonds. the video seems to be a cooking tutorial, with the woman guiding the viewers through the preparation and use of almonds in various dishes.

**SUM-holistic** video summarization:

the video begins with a woman in a well-equipped kitchen, addressing the camera with a smile. she is wearing a green t-shirt and is surrounded by brown wooden cabinets and appliances. as she speaks, she reveals that there are a few tricks that people need to know in order to be successful. the scene transitions to a close-up of a clear, transparent blender. the woman's voice instructs viewers to roast their almonds to bring out not only the flavors but the oil as well. the video then shifts back to the woman in the kitchen, now holding the transparent blender. she continues to speak to the camera, emphasizing the importance of roasting the almonds. in the final scene, the woman is seen using a wooden spatula to scoop up the roasted almonds from a baking tray. she then places the tray in the oven to continue roasting the nuts. throughout the video, the woman's words and actions provide a comprehensive guide on how to successfully roast almonds.

**SUM-shot** video summarization:

the video begins with a woman in a kitchen setting, wearing a blue top and blonde hair. she is holding a clear plastic container in her hands, which contains almonds. as she speaks to the camera, she mentions a couple of tricks that people need to know in order to be successful. the scene transitions to a close-up of a plate of almonds being cooked in an oven using a shovel. the woman's voice can be heard in the background, explaining that roasting the almonds helps to bring out not only the flavors but the oil as well. in the final scene, the woman continues to hold the clear plastic container filled with almonds. she is seated in a well-equipped kitchen, with a blender placed next to her. as she speaks to the camera, she holds a bowl of almonds in her other hand. the video seems to be a tutorial or a cooking demonstration, with the woman sharing her knowledge and tips on roasting almonds.

**Ground truth** video summary:

the video begins with a woman, dressed in green short sleeves, standing in front of a kitchen console. she is engaged in a conversation, presumably about cooking tips, as she stands next to a bowl of almonds and a transparent mixer. as she speaks, she picks up the bowl of almonds, emphasizing the importance of knowing certain tricks for successful cooking. the scene transitions smoothly to a close-up of an oven pan filled with almonds. a wooden spoon is used to stir the almonds around in the pan. the woman's voice continues in the background, explaining the benefits of roasting almonds. she mentions that this process helps to enhance the flavors of the almonds, suggesting that this is one of the tricks she was referring to earlier. the video concludes with the woman once again standing in front of the kitchen console, continuing her discussion. she holds the bowl of almonds in her hands, possibly preparing to demonstrate the next step in her cooking process. throughout the video, the woman's actions and dialogue suggest that she is sharing her knowledge and tips about cooking, specifically focusing on the use of almonds.



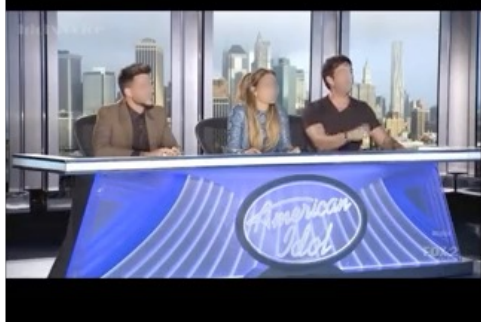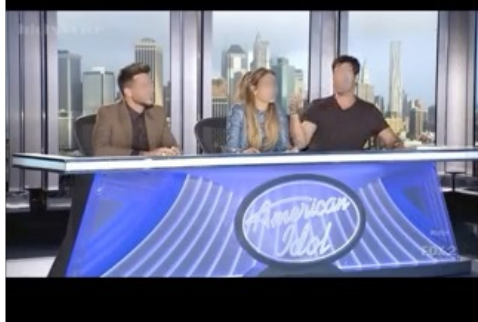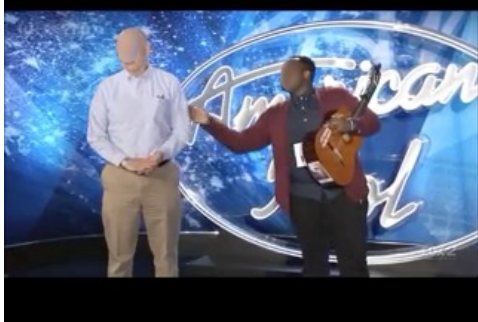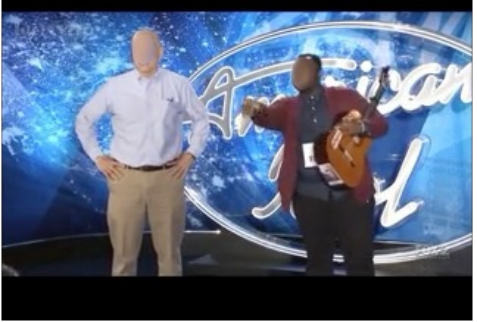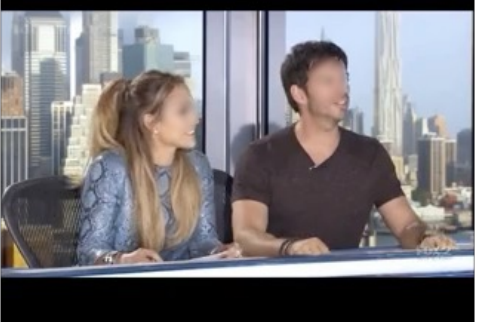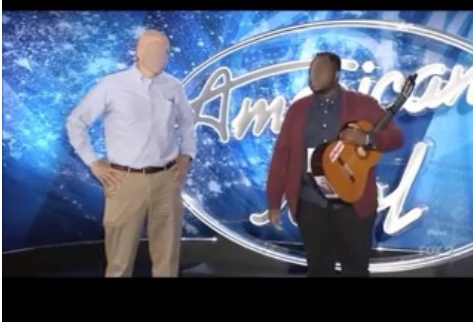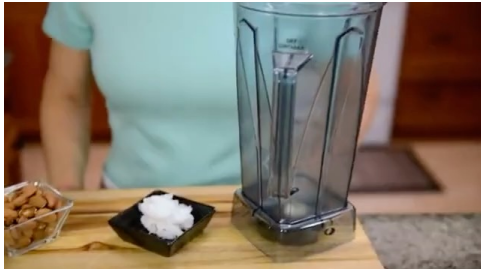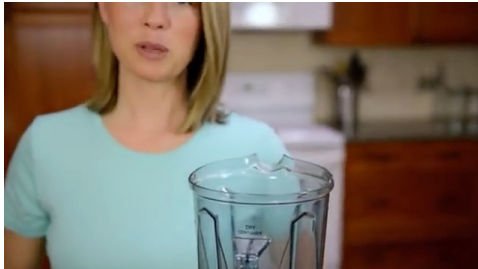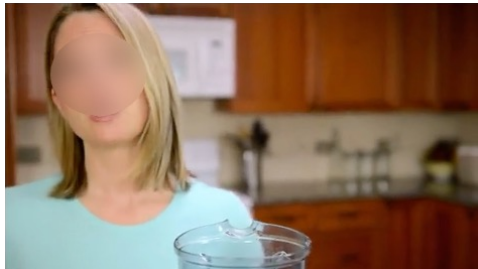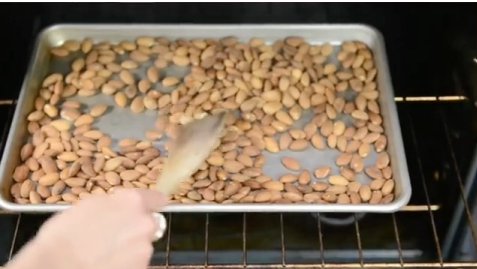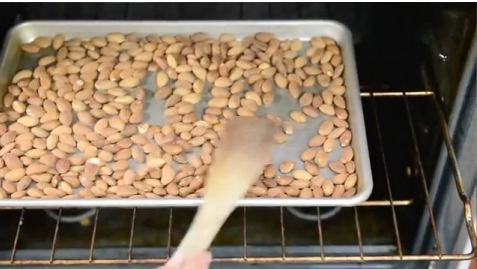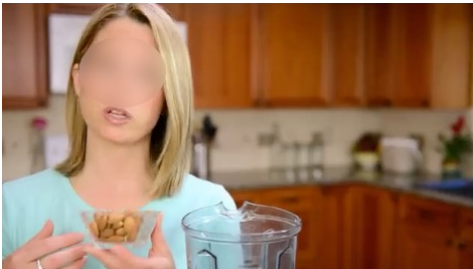

Supplement: Supplementary file 8 [file supp_sum_summary_sample1.pdf]
